# Supplementary material for: Self-Supervised Learning Disentangled Group Representation as Feature
Source: arXiv:2110.15255 source file (2021-10-29)
Supplement: Supplementary file 1 [file abstract.tex]

%\begin{abstract}

%\end{abstract}
