# Supplementary material for: Self-Supervised Learning Disentangled Group Representation as Feature
Source: arXiv:2110.15255 source file (2021-10-29)

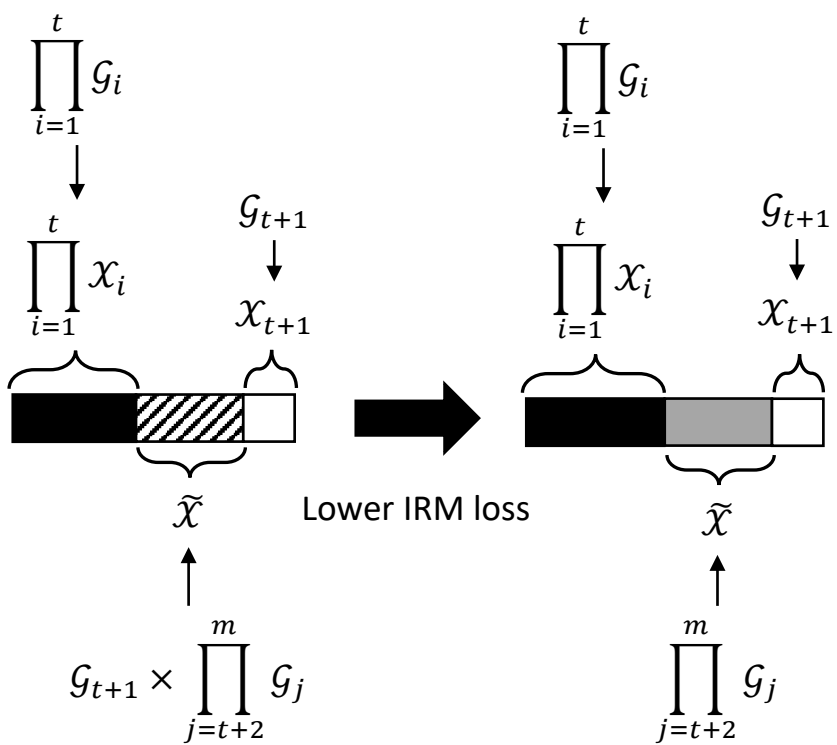

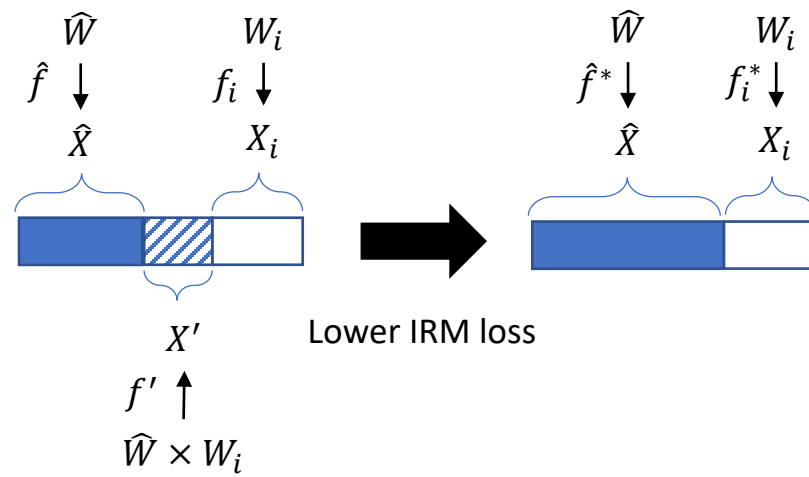

Supplement: Supplementary file 2 [file IRM_minimization.pdf]
